# Supplementary material for: From Shallow Bayesian Neural Networks to Gaussian Processes: General Convergence, Identifiability and Scalable Inference
Source: arXiv:2602.22492 source file (2026-02-26)
Supplement: Supplementary file 1 [file supplementary.pdf]

# Supplementary Material for
From Shallow Bayesian Neural Networks to Gaussian Processes: General Convergence, Identifiability, and Scalable MAP Inference via Nyström

Gracielle Antunes de Araújo    Flávio B. Gonçalves

**Contents.** This supplementary material includes: (i) technical details and proofs; (ii) additional derivations for activation-induced kernels; (iii) computational details for MAP estimation via Nyström; and (iv) extended experimental tables and protocols omitted from the main paper due to space.

## S1 Technical details and proofs

### S1.1 Pre-activation moments and dependence across inputs

For a fixed hidden unit $j$, consider the pre-activations $z(\mathbf{x}) = a + \mathbf{u}^\top \mathbf{x}, z(\mathbf{x}') = a + \mathbf{u}^\top \mathbf{x}'$, where $a$ and $\mathbf{u}$ are drawn from the parameter *prioris* (with zero mean and finite variances). Under the assumptions in the main text, we have:

**Mean.**

$$\mathbb{E}[z(\mathbf{x})] = \mathbb{E}[a] + \sum_{i=1}^{I} x_i \mathbb{E}[u_i] = 0, \qquad \mathbb{E}[z(\mathbf{x}')] = 0.$$

**Variance.** Assuming independence between $a$ and $\mathbf{u}$, and finite variances,

$$\mathrm{Var}(z(\mathbf{x})) = \mathrm{Var}(a) + \mathrm{Var}(\mathbf{u}^\top \mathbf{x}) = \sigma_a^2 + \sigma_u^2\, \mathbf{x}^\top \mathbf{x},$$

and similarly $\mathrm{Var}(z(\mathbf{x}')) = \sigma_a^2 + \sigma_u^2\, \mathbf{x}'^\top \mathbf{x}'$.

**Covariance.** Note that $z(\mathbf{x})$ and $z(\mathbf{x}')$ are *not* independent: they share the same $a$ and the same $\mathbf{u}$. Their covariance is

$$\mathrm{Cov}(z(\mathbf{x}), z(\mathbf{x}')) = \mathrm{Var}(a) + \mathrm{Cov}(\mathbf{u}^\top \mathbf{x}, \mathbf{u}^\top \mathbf{x}') = \sigma_a^2 + \sigma_u^2\, \mathbf{x}^\top \mathbf{x}'.$$

In particular, when $a$ and $\mathbf{u}$ are Gaussian, $(z(\mathbf{x}), z(\mathbf{x}'))$ is a centered bivariate Gaussian with covariance matrix determined by the quantities above.

### S1.2 A general regularity condition

We next state a simple sufficient condition ensuring $\mathbb{E}[h(Z)^2] < \infty$ when $Z$ is Gaussian.

*Proposition* S1.1 (Polynomial growth implies a finite second moment). If $h : \mathbb{R} \to \mathbb{R}$ satisfies $|h(z)| \le C(1 + |z|^p)$ for some $C > 0$ and $p \ge 0$, then for $Z \sim \mathcal{N}(0, \sigma^2)$ we have $\mathbb{E}[h(Z)^2] < \infty$.

*Proof.* By assumption, $h(Z)^2 \le 2C^2(1 + |Z|^{2p})$. Since Gaussian random variables have moments of all orders, $\mathbb{E}[|Z|^{2p}] < \infty$. Hence, $\mathbb{E}[h(Z)^2] \le 2C^2(1 + \mathbb{E}[|Z|^{2p}]) < \infty$. □

### S1.3 Extension to deep networks

Although our focus is on shallow networks, the same phenomenon holds for deep architectures under infinite width in all hidden layers: finite-dimensional distributions converge to Gaussians and the kernel is obtained recursively (Novak et al., 2020; Lee et al., 2018). Consider a feedforward network with $L$ layers and define

$$\begin{aligned}
\mathbf{h}^{(0)}(\mathbf{x}) &= \mathbf{x}, \\
\mathbf{z}^{(\ell)}(\mathbf{x}) &= W^{(\ell)}\,\mathbf{h}^{(\ell-1)}(\mathbf{x}) + \mathbf{b}^{(\ell)}, \qquad \ell = 1, \ldots, L, \\
\mathbf{h}^{(\ell)}(\mathbf{x}) &= h\big(\mathbf{z}^{(\ell)}(\mathbf{x})\big), \qquad \ell = 1, \ldots, L-1, \\
\mathbf{f}(\mathbf{x}) &= g\big(\mathbf{z}^{(L)}(\mathbf{x})\big).
\end{aligned} \tag{1}$$

Under i.i.d. Gaussian initialization,

$$W_{ji}^{(\ell)} \sim \mathcal{N}\left(0, \frac{\sigma_w^2}{H_{\ell-1}}\right), \qquad b_j^{(\ell)} \sim \mathcal{N}(0, \sigma_b^2),$$

as $H_1, \ldots, H_{L-1} \to \infty$ one obtains a GP whose kernel is computed by a depth recursion. Define $K^{(0)}(\mathbf{x}, \mathbf{x}') = \frac{1}{I}\mathbf{x}^\top \mathbf{x}'$ and $\Sigma^{(0)}(\mathbf{x}, \mathbf{x}') = \sigma_b^2 + \sigma_w^2 K^{(0)}(\mathbf{x}, \mathbf{x}')$. For $\ell \geq 0$,

$$\Sigma^{(\ell)}(\mathbf{x}, \mathbf{x}') = \sigma_b^2 + \sigma_w^2 K^{(\ell)}(\mathbf{x}, \mathbf{x}'), \tag{2}$$

$$K^{(\ell+1)}(\mathbf{x}, \mathbf{x}') = \mathbb{E}\big[h(Z)\,h(Z')\big], \tag{3}$$

where $(Z, Z')$ is a centered bivariate Gaussian with covariance determined by $\Sigma^{(\ell)}$. Finally, the output covariance takes the form

$$\mathrm{Cov}\left(f(\mathbf{x}), f(\mathbf{x}')\right) = \sigma_b^2 + \sigma_w^2 K^{(L)}(\mathbf{x}, \mathbf{x}').$$

## S2 Kernel derivations

### S2.1 Calculations of the terms $\mathbb{E}[h(Z)\,h(Z')]$ for common activations

In this subsection we detail the calculations (and standard approximations) for the inner term $\mathbb{E}[h(Z)h(Z')]$ when $(Z, Z')$ is a centered bivariate Gaussian. This term determines the induced kernel in the infinite-width limit:

$$K_h(\mathbf{x}, \mathbf{x}') = \sigma_b^2 + \sigma_v^2\,\mathbb{E}[h(Z)\,h(Z')].$$

Throughout this subsection, we assume that $(Z, Z')$ has standard deviations $\sigma_z, \sigma_{z'} > 0$ and correlation $\rho \in (-1, 1)$. Thus,

$$\mathbb{E}[h(Z)h(Z')] = \iint_{\mathbb{R}^2} h(z)\,h(z')\;\phi_{\rho,\sigma_z,\sigma_{z'}}(z, z')\,dz\,dz', \tag{4}$$

where $\phi_{\rho,\sigma_z,\sigma_{z'}}$ is the bivariate Normal density with zero means, standard deviations $\sigma_z, \sigma_{z'}$, and correlation $\rho$.

**Standardization.** Write $Z = \sigma_z U$ and $Z' = \sigma_{z'} V$, where $(U, V)$ is a standard bivariate Normal with $\mathrm{Corr}(U, V) = \rho$. Then (4) is equivalent to

$$\mathbb{E}[h(Z)h(Z')] = \mathbb{E}\big[h(\sigma_z U)\,h(\sigma_{z'} V)\big], \qquad (U, V) \sim \mathcal{N}\left(\mathbf{0}, \begin{bmatrix} 1 & \rho \\ \rho & 1 \end{bmatrix}\right). \tag{5}$$

### S2.1.1 Product of erf functions

The calculations for tanh and the sigmoid below use the following classical result.

**Lemma S2.1** (erf × erf identity)**.** *If* $(U, V)$ *is a standard bivariate Normal with* $\mathrm{Corr}(U, V) = \rho$*, then for* $A, B \in \mathbb{R}$*,*

$$\mathbb{E}[\mathrm{erf}(AU)\,\mathrm{erf}(BV)] = \frac{2}{\pi}\arcsin\left(\frac{2AB\,\rho}{\sqrt{(1+2A^2)(1+2B^2)}}\right). \tag{6}$$

*Proof.* A classical proof uses the integral representation $\mathrm{erf}(t) = \frac{2}{\sqrt{\pi}}\int_0^t e^{-s^2}\,ds$ and Fubini's theorem to rewrite the expectation as a double integral involving Gaussian probabilities. Another (also standard) route uses the identity $\mathrm{erf}(t) = 2\Phi(\sqrt{2}\,t) - 1$, where $\Phi$ is the standard Normal CDF, and reduces $\mathbb{E}[\Phi(\cdot)\Phi(\cdot)]$ to a tractable bivariate integral. The final expression (6) is well documented in the infinite-width neural network kernel literature (see Williams (1997); Rasmussen and Williams (2006)). □

### S2.1.2 Activation tanh

The expectation

$$\mathbb{E}[\tanh(Z)\tanh(Z')] = \iint_{\mathbb{R}^2} \tanh(z)\tanh(z')\,\phi_{\rho,\sigma_z,\sigma_{z'}}(z, z')\,dz\,dz' \tag{7}$$

does not admit a simple closed form. Following Williams (1997), we use the standard approximation

$$\tanh(x) \approx \mathrm{erf}\left(\frac{\sqrt{\pi}}{2}\,x\right). \tag{8}$$

**Standardization and application of the lemma.** Since $(Z, Z')$ is a centered bivariate Normal with standard deviations $\sigma_z, \sigma_{z'}$ and correlation $\rho$, we may write

$$Z = \sigma_z U, \qquad Z' = \sigma_{z'} V,$$

where $(U, V)$ is a *standard* bivariate Normal with $\mathrm{Corr}(U, V) = \rho$. Substituting (8) into (7) yields

$$\begin{aligned}\mathbb{E}[\tanh(Z)\tanh(Z')] &\approx \mathbb{E}\left[\mathrm{erf}\left(\frac{\sqrt{\pi}}{2}\,Z\right)\,\mathrm{erf}\left(\frac{\sqrt{\pi}}{2}\,Z'\right)\right] \\ &= \mathbb{E}[\mathrm{erf}(AU)\,\mathrm{erf}(BV)]\,,\end{aligned} \tag{9}$$

with

$$A = \frac{\sqrt{\pi}}{2}\,\sigma_z, \qquad B = \frac{\sqrt{\pi}}{2}\,\sigma_{z'}.$$

Applying Lemma S2.1 to (9) gives

$$\begin{aligned}\mathbb{E}[\tanh(Z)\tanh(Z')] &\approx \frac{2}{\pi}\arcsin\left(\frac{2AB\,\rho}{\sqrt{(1+2A^2)(1+2B^2)}}\right) \\ &= \frac{2}{\pi}\arcsin\left(\frac{\frac{\pi}{2}\,\sigma_z\sigma_{z'}\,\rho}{\sqrt{\left(1+\frac{\pi}{2}\sigma_z^2\right)\left(1+\frac{\pi}{2}\sigma_{z'}^2\right)}}\right).\end{aligned} \tag{10}$$

Therefore, the induced (infinite-width) kernel is

$$K_{\tanh}(\mathbf{x}, \mathbf{x}') = \sigma_b^2 + \sigma_v^2\,\frac{2}{\pi}\arcsin\left(\frac{\frac{\pi}{2}\,\sigma_z\sigma_{z'}\,\rho}{\sqrt{\left(1+\frac{\pi}{2}\sigma_z^2\right)\left(1+\frac{\pi}{2}\sigma_{z'}^2\right)}}\right). \tag{11}$$

**Comment (accuracy of the approximation).** The approximation (8) is particularly accurate for $x \approx 0$ and for $|x| \to \infty$. Indeed, comparing the Taylor expansions around 0,

$$\tanh(x) = x - \frac{x^3}{3} + \mathcal{O}(x^5), \qquad \operatorname{erf}\left(\frac{\sqrt{\pi}}{2}x\right) = x - \frac{\pi}{12}x^3 + \mathcal{O}(x^5),$$

so the error is $\mathcal{O}(x^3)$ as $x \to 0$, and both functions tend to $\pm 1$ as $|x| \to \infty$.

### S2.1.3 Sigmoid activation

We derive an approximate closed-form expression for the inner term $\mathbb{E}[\mathrm{sigmoid}(Z)\mathrm{sigmoid}(Z')]$ by rewriting the sigmoid in terms of tanh and then applying the same tanh $\approx$ erf approximation used in the previous subsection. Recall the exact identity

$$\mathrm{sigmoid}(z) = \frac{1}{1+e^{-z}} = \frac{1}{2}\left(1 + \tanh\left(\frac{z}{2}\right)\right).$$

Hence, by linearity of expectation,

$$\begin{aligned}\mathbb{E}[\mathrm{sigmoid}(Z)\mathrm{sigmoid}(Z')] &= \frac{1}{4}\,\mathbb{E}\Big[\Big(1+\tanh\big(\tfrac{Z}{2}\big)\Big)\Big(1+\tanh\big(\tfrac{Z'}{2}\big)\Big)\Big] \\ &= \frac{1}{4}\,\mathbb{E}\Big[1+\tanh\big(\tfrac{Z}{2}\big)+\tanh\big(\tfrac{Z'}{2}\big)+\tanh\big(\tfrac{Z}{2}\big)\tanh\big(\tfrac{Z'}{2}\big)\Big].\end{aligned}$$

Since $(Z, Z')$ is centered Gaussian and tanh is an odd function, symmetry yields $\mathbb{E}[\tanh(Z/2)] = \mathbb{E}[\tanh(Z'/2)] = 0$. Therefore,

$$\mathbb{E}[\mathrm{sigmoid}(Z)\mathrm{sigmoid}(Z')] = \frac{1}{4} + \frac{1}{4}\,\mathbb{E}\left[\tanh\left(\frac{Z}{2}\right)\tanh\left(\frac{Z'}{2}\right)\right]. \tag{12}$$

Next, we use the standard approximation (as in Williams (1997))

$$\tanh(x) \approx \operatorname{erf}\left(\frac{\sqrt{\pi}}{2}\,x\right), \qquad \Rightarrow \qquad \tanh\left(\frac{z}{2}\right) \approx \operatorname{erf}\left(\frac{\sqrt{\pi}}{4}\,z\right).$$

Write $Z = \sigma_z U$ and $Z' = \sigma_{z'} V$, where $(U, V)$ is standard bivariate normal with $\mathrm{Corr}(U, V) = \rho$. Setting

$$A = \frac{\sqrt{\pi}}{4}\sigma_z, \qquad B = \frac{\sqrt{\pi}}{4}\sigma_{z'},$$

we obtain

$$\mathbb{E}\left[\tanh\left(\frac{Z}{2}\right)\tanh\left(\frac{Z'}{2}\right)\right] \approx \mathbb{E}\big[\operatorname{erf}(AU)\operatorname{erf}(BV)\big].$$

Applying Lemma S2.1 (erf$\times$erf identity) gives

$$\mathbb{E}\big[\operatorname{erf}(AU)\operatorname{erf}(BV)\big] = \frac{2}{\pi}\arcsin\left(\frac{2AB\,\rho}{\sqrt{(1+2A^2)(1+2B^2)}}\right).$$

Substituting $A, B$ yields $2AB = \frac{\pi}{8}\sigma_z\sigma_{z'}$, $1 + 2A^2 = 1 + \frac{\pi}{8}\sigma_z^2$, and $1 + 2B^2 = 1 + \frac{\pi}{8}\sigma_{z'}^2$, so

$$\mathbb{E}[\mathrm{sigmoid}(Z)\mathrm{sigmoid}(Z')] \approx \frac{1}{4} + \frac{1}{2\pi}\arcsin\left(\frac{\frac{\pi}{8}\,\sigma_z\sigma_{z'}\,\rho}{\sqrt{\left(1+\frac{\pi}{8}\sigma_z^2\right)\left(1+\frac{\pi}{8}\sigma_{z'}^2\right)}}\right). \tag{13}$$

Finally, substituting into $K_{\text{sig}}(\mathbf{x}, \mathbf{x}') = \sigma_b^2 + \sigma_v^2\,\mathbb{E}[\text{sigmoid}(Z)\text{sigmoid}(Z')]$, we obtain

$$K_{\text{sig}}(\mathbf{x}, \mathbf{x}') = \sigma_b^2 + \sigma_v^2 \left[ \frac{1}{4} + \frac{1}{2\pi} \arcsin\!\left( \frac{\frac{\pi}{8}\,\sigma_z \sigma_{z'}\,\rho}{\sqrt{\left(1 + \frac{\pi}{8}\sigma_z^2\right)\left(1 + \frac{\pi}{8}\sigma_{z'}^2\right)}} \right) \right]. \tag{14}$$

#### S2.1.4 Activation ReLU

Let $h(z) = \text{ReLU}(z) = \max(0, z) = z\,\mathbf{1}_{\{z>0\}}$. Then

$$\text{ReLU}(Z)\text{ReLU}(Z') = ZZ'\,\mathbf{1}_{\{Z>0,Z'>0\}},$$

and therefore

$$\mathbb{E}[\text{ReLU}(Z)\text{ReLU}(Z')] = \mathbb{E}\big[ZZ'\,\mathbf{1}_{\{Z>0,Z'>0\}}\big]. \tag{15}$$

**Standardization.** Write $Z = \sigma_z U$ and $Z' = \sigma_{z'} V$, where $(U, V)$ is a standard bivariate Normal with $\text{Corr}(U, V) = \rho$. Then (15) becomes

$$\mathbb{E}[\text{ReLU}(Z)\text{ReLU}(Z')] = \sigma_z \sigma_{z'}\,\mathbb{E}\big[UV\,\mathbf{1}_{\{U>0,V>0\}}\big]. \tag{16}$$

**Computing $\mathbb{E}[UV\,\mathbf{1}_{\{U>0,V>0\}}]$.** Use the standard representation

$$V = \rho U + \sqrt{1 - \rho^2}\,E, \qquad E \sim \mathcal{N}(0, 1),\ \ E \perp U.$$

Conditioning on $U = u > 0$, we have $V \mid U = u \sim \mathcal{N}(\rho u,\, 1 - \rho^2)$. For a Normal random variable $X \sim \mathcal{N}(\mu, \sigma^2)$, the truncated first moment satisfies

$$\mathbb{E}[X\,\mathbf{1}_{\{X>0\}}] = \mu\,\Phi(\mu/\sigma) + \sigma\,\varphi(\mu/\sigma), \tag{17}$$

where $\Phi$ and $\varphi$ are the standard Normal cdf and pdf. Applying (17) with $\mu = \rho u$ and $\sigma = \sqrt{1 - \rho^2}$ gives

$$\mathbb{E}[V\,\mathbf{1}_{\{V>0\}} \mid U = u] = \rho u\,\Phi(\kappa u) + \sqrt{1 - \rho^2}\,\varphi(\kappa u), \qquad \kappa := \frac{\rho}{\sqrt{1 - \rho^2}}.$$

Hence,

$$\begin{aligned}
\mathbb{E}\big[UV\,\mathbf{1}_{\{U>0,V>0\}}\big] &= \int_0^\infty u\,\varphi(u)\,\mathbb{E}[V\,\mathbf{1}_{\{V>0\}} \mid U = u]\ du \\
&= \rho \int_0^\infty u^2\,\varphi(u)\,\Phi(\kappa u)\,du \ + \ \sqrt{1 - \rho^2} \int_0^\infty u\,\varphi(u)\,\varphi(\kappa u)\,du. \qquad (18)
\end{aligned}$$

The two integrals in (18) have closed forms (they can be derived by standard calculus; see, e.g., Neal (1996); Williams (1997)):

$$\int_0^\infty u\,\varphi(u)\,\varphi(\kappa u)\,du = \frac{1}{2\pi}\,\frac{1}{1 + \kappa^2} = \frac{1}{2\pi}\,(1 - \rho^2), \tag{19}$$

$$\int_0^\infty u^2\,\varphi(u)\,\Phi(\kappa u)\,du = \frac{1}{2\pi}\Big(\frac{\pi}{2} + \arctan(\kappa)\Big) = \frac{1}{2\pi}(\pi - \arccos(\rho)), \tag{20}$$

where we used $\arctan(\kappa) = \arcsin(\rho)$ and $\arcsin(\rho) + \arccos(\rho) = \pi/2$. Substituting (19)–(20) into (18) yields

$$\mathbb{E}\big[UV\,\mathbf{1}_{\{U>0,V>0\}}\big] = \frac{1}{2\pi}\Big[\sqrt{1 - \rho^2} + \rho(\pi - \arccos(\rho))\Big]. \tag{21}$$

Combining (16) and (21), we obtain

$$\mathbb{E}[\mathrm{ReLU}(Z)\mathrm{ReLU}(Z')] = \frac{\sigma_z \sigma_{z'}}{2\pi}\Big[\sqrt{1-\rho^2} + \rho(\pi - \arccos(\rho))\Big]. \tag{22}$$

Therefore, the induced (infinite-width) kernel is

$$K_{\mathrm{ReLU}}(\mathbf{x}, \mathbf{x}') = \sigma_b^2 + \sigma_v^2 \frac{\sigma_z \sigma_{z'}}{2\pi}\Big[\sqrt{1-\rho^2} + \rho(\pi - \arccos(\rho))\Big]. \tag{23}$$

**Comment.** Equation (22) is the classical *arccos kernel.* The derivation above makes explicit the key steps: standardization, conditioning $V \mid U = u$, the truncated Normal moment (17), and the resulting one-dimensional integrals leading to (21).

### S2.1.5 Activation LeakyReLU

Let

$$\mathrm{LeakyReLU}(z) = \begin{cases} z, & z \geq 0, \\ \alpha z, & z < 0, \end{cases} \qquad 0 < \alpha < 1.$$

A convenient identity is the decomposition in terms of ReLU:

$$\mathrm{LeakyReLU}(z) = \alpha z + (1-\alpha)\mathrm{ReLU}(z), \qquad \mathrm{ReLU}(z) = z\,\mathbf{1}_{\{z>0\}}. \tag{24}$$

By expanding the product, we obtain four terms:

$$\begin{aligned}\mathrm{LeakyReLU}(z)\,\mathrm{LeakyReLU}(z') = &\underbrace{\alpha^2\, z\, z'}_{\text{(A)}} + \underbrace{\alpha(1-\alpha)\, z\, \mathrm{ReLU}(z')}_{\text{(B)}} \\ &+ \underbrace{\alpha(1-\alpha)\, z'\, \mathrm{ReLU}(z)}_{\text{(C)}} + \underbrace{(1-\alpha)^2\, \mathrm{ReLU}(z)\, \mathrm{ReLU}(z')}_{\text{(D)}}.\end{aligned}$$

Hence,

$$\begin{aligned}\mathbb{E}\big[\mathrm{LeakyReLU}(z)\,\mathrm{LeakyReLU}(z')\big] &= \alpha^2\, \mathbb{E}[z\, z'] + \alpha(1-\alpha)\, \mathbb{E}\big[z\, \mathrm{ReLU}(z')\big] \\ &\quad + \alpha(1-\alpha)\, \mathbb{E}\big[z'\, \mathrm{ReLU}(z)\big] \\ &\quad + (1-\alpha)^2\, \mathbb{E}\big[\mathrm{ReLU}(z)\, \mathrm{ReLU}(z')\big]. \end{aligned} \tag{25}$$

**Term 1: $\mathbb{E}[ZZ']$.** Since $(Z, Z')$ is centered with $\mathrm{Corr}(Z, Z') = \rho$ and standard deviations $\sigma_z, \sigma_{z'}$,

$$\mathbb{E}[ZZ'] = \mathrm{Cov}(Z, Z') = \rho\, \sigma_z \sigma_{z'}. \tag{26}$$

**Term 2: $\mathbb{E}[Z\, \mathrm{ReLU}(Z')]$.** Write $Z = \sigma_z U$ and $Z' = \sigma_{z'} V$, where $(U, V)$ is a standard bivariate Normal with correlation $\rho$. Then

$$\mathbb{E}[Z\, \mathrm{ReLU}(Z')] = \sigma_z \sigma_{z'}\, \mathbb{E}[U\, V\, \mathbf{1}_{\{V>0\}}].$$

Using conditional expectation, $\mathbb{E}[U \mid V] = \rho V$, hence

$$\mathbb{E}[U\, V\, \mathbf{1}_{\{V>0\}}] = \mathbb{E}[\mathbb{E}[U \mid V]\; V\, \mathbf{1}_{\{V>0\}}] = \rho\, \mathbb{E}[V^2 \mathbf{1}_{\{V>0\}}].$$

Since $V^2$ is even and $\mathbb{P}(V > 0) = 1/2$, we have $\mathbb{E}[V^2 \mathbf{1}_{\{V>0\}}] = \frac{1}{2}\mathbb{E}[V^2] = \frac{1}{2}$, so

$$\mathbb{E}[Z\, \mathrm{ReLU}(Z')] = \frac{\rho\, \sigma_z \sigma_{z'}}{2}. \tag{27}$$

**Term 3:** $\mathbb{E}[\mathrm{ReLU}(Z)\mathrm{ReLU}(Z')]$**.** From the ReLU case,

$$\mathbb{E}[\mathrm{ReLU}(Z)\mathrm{ReLU}(Z')] = \frac{\sigma_z \sigma_{z'}}{2\pi}\Big[\sqrt{1-\rho^2} + \rho(\pi - \arccos(\rho))\Big]. \tag{28}$$

**Putting terms together.** Substituting (26), (27) and (28) into (25), we get

$$\begin{aligned}\mathbb{E}\big[\mathrm{LeakyReLU}(z)\,\mathrm{LeakyReLU}(z')\big] &= \alpha^2\,\rho\,\sigma_z\,\sigma_{z'} \\ &\quad + \alpha(1-\alpha)\left(\frac{\rho\,\sigma_z\,\sigma_{z'}}{2} + \frac{\rho\,\sigma_z\,\sigma_{z'}}{2}\right) \\ &\quad + (1-\alpha)^2\,\sigma_z\,\sigma_{z'}\,\frac{1}{2\pi}\left[\sqrt{1-\rho^2} + \rho(\pi - \arccos(\rho))\right]. \end{aligned} \tag{29}$$

where

$$S(\rho) := \frac{1}{2\pi}\Big[\sqrt{1-\rho^2} + \rho(\pi - \arccos(\rho))\Big]. \tag{30}$$

Therefore the induced (infinite-width) kernel is

$$K_{\mathrm{LeakyReLU}}(\mathbf{x}, \mathbf{x}') = \sigma_b^2 + \sigma_v^2\,\sigma_z\sigma_{z'}\Big[\alpha\,\rho + (1-\alpha)^2\,S(\rho)\Big]. \tag{31}$$

Note that (31) reduces to the ReLU kernel when $\alpha = 0$.

## S2.2 Practical identifiability under i.i.d. designs and stratification

This section provides supporting calculations for Section 4.4. The key phenomenon is that, in high dimension, i.i.d. sampling induces concentration of both norms and angles, which restricts the effective range of kernel evaluations and may render theoretical identifiability numerically fragile.

### S2.2.1 Concentration under i.i.d. designs

**Setup.** Let $\mathbf{x}, \mathbf{x}' \in [0,1]^I$ be independent random vectors. Write

$$u(\mathbf{x}) = \|\mathbf{x}\|^2 = \sum_{j=1}^{I} x_j^2, \qquad \mathbf{x}^\top\mathbf{x}' = \sum_{j=1}^{I} x_j x_j', \qquad \tilde{\rho}(\mathbf{x}, \mathbf{x}') = \frac{\mathbf{x}^\top\mathbf{x}'}{\|\mathbf{x}\|\|\mathbf{x}'\|}.$$

**Uniform case ($x_j \overset{i.i.d.}{\sim} \mathrm{Unif}(0,1)$).** By the law of large numbers,

$$\frac{u(\mathbf{x})}{I} \xrightarrow{\text{a.s.}} \mathbb{E}[X^2] = \frac{1}{3}, \qquad \frac{\mathbf{x}^\top\mathbf{x}'}{I} \xrightarrow{\text{a.s.}} \mathbb{E}[X]\mathbb{E}[X'] = \frac{1}{4}.$$

Moreover,

$$\mathrm{Var}(X^2) = \mathbb{E}[X^4] - \mathbb{E}[X^2]^2 = \frac{1}{5} - \Big(\frac{1}{3}\Big)^2 = \frac{4}{45}, \qquad \mathrm{Var}(XX') = \frac{1}{9} - \frac{1}{16} = \frac{7}{144}.$$

Thus,

$$\mathrm{Var}\Big(\frac{u(\mathbf{x})}{I}\Big) = \frac{4}{45}\cdot\frac{1}{I}, \qquad \mathrm{Var}\Big(\frac{\mathbf{x}^\top\mathbf{x}'}{I}\Big) = \frac{7}{144}\cdot\frac{1}{I},$$

i.e., typical fluctuations shrink as $O(I^{-1/2})$. Finally, by Slutsky's theorem,

$$\tilde{\rho}(\mathbf{x}, \mathbf{x}') = \frac{\frac{\mathbf{x}^\top\mathbf{x}'}{I}}{\sqrt{\frac{u(\mathbf{x})}{I}\cdot\frac{u(\mathbf{x}')}{I}}} \xrightarrow{\mathbb{P}} \frac{\frac{1}{4}}{\sqrt{(\frac{1}{3})(\frac{1}{3})}} = \frac{3}{4}.$$

**General i.i.d. inputs with finite moments.** The same mechanism holds more generally. If $\mathbf{x} = (x_1, \ldots, x_I)$ has i.i.d. coordinates with $\mathbb{E}[x_1^2] < \infty$, then

$$\frac{\|\mathbf{x}\|^2}{I} = \frac{1}{I}\sum_{j=1}^{I} x_j^2 \xrightarrow{\text{a.s.}} \mathbb{E}[x_1^2].$$

If $\mathbf{x}$ and $\mathbf{x}'$ are independent with $\mathbb{E}[|x_1|] < \infty$, then

$$\frac{\mathbf{x}^\top \mathbf{x}'}{I} = \frac{1}{I}\sum_{j=1}^{I} x_j x_j' \xrightarrow{\text{a.s.}} \mathbb{E}[x_1]\mathbb{E}[x_1'].$$

When fourth moments exist, the variances of these averages scale as $O(I^{-1})$, implying $O(I^{-1/2})$ fluctuations. Therefore, numerical fragility of identification is driven primarily by the combination of high dimension and i.i.d. sampling, rather than by the specific Uniform distribution.

### S2.2.2 Radial information and conditioning of the pre-activation variance parameters

For the mixed kernel, the diagonal depends on $\mathbf{x}$ through $\sigma_z^2(\mathbf{x}) = \sigma_u^2\|\mathbf{x}\|^2 + \sigma_a^2$. Let $r_i^2 = \|\mathbf{x}_i\|^2$ and consider the linear form

$$s_i = \sigma_u^2 r_i^2 + \sigma_a^2.$$

Writing $\boldsymbol{\phi}_i = (r_i^2, 1)^\top$, define the empirical second-moment (Gram) matrix

$$\mathbf{G} = \frac{1}{n}\sum_{i=1}^{n} \boldsymbol{\phi}_i \boldsymbol{\phi}_i^\top = \frac{1}{n}\sum_{i=1}^{n} \begin{bmatrix} r_i^4 & r_i^2 \\ r_i^2 & 1 \end{bmatrix}.$$

A direct computation yields

$$\det(\mathbf{G}) = \Big(\tfrac{1}{n}\sum_{i=1}^{n} r_i^4\Big) - \Big(\tfrac{1}{n}\sum_{i=1}^{n} r_i^2\Big)^2 = \mathrm{Var}_n(r^2).$$

Hence, when $\mathrm{Var}_n(r^2)$ is small (as under i.i.d. designs in high dimension), the separation of $(\sigma_u^2, \sigma_a^2)$ becomes numerically ill-conditioned.

**Radial stratification.** Let $R = r^2/I$ and consider a two-stratum construction: draw $S \in \{0, 1\}$ with $\mathbb{P}(S = 1) = p$, and impose

$$\mathbb{E}[R \mid S = 0] = a, \quad \mathrm{Var}(R \mid S = 0) = \tau_0^2, \qquad \mathbb{E}[R \mid S = 1] = b, \quad \mathrm{Var}(R \mid S = 1) = \tau_1^2,$$

with $b > a$. By the law of total variance,

$$\mathrm{Var}(R) = (1-p)\tau_0^2 + p\tau_1^2 + p(1-p)(b-a)^2 \approx p(1-p)(b-a)^2 > 0,$$

when intra-stratum variances are small. Since $r^2 = IR$, this preserves dispersion in $r^2$ and stabilizes diagonal-based identification.

### S2.2.3 Angular stratification

To separate the smooth term $A(\rho)$ from the angular term $B(\rho; \alpha)$, it is necessary to observe kernel evaluations over a range of correlations. In simulations, we implement angular stratification by placing a fraction of points near multiple corners of $\{0, 1\}^I$, which generates pairs with low, intermediate, and high cosine similarities, thereby improving the numerical separation of kernel components.

#### S2.2.4 Illustrative quantiles

Table S1: Empirical quantiles of $r^2/I$ and cosine similarity $\tilde{\rho}(\mathbf{x}, \mathbf{x}')$ (illustrative example, $I = 10$).

| Design | $r^2/I$ | | | $\tilde{\rho}(\mathbf{x}, \mathbf{x}')$ | | |
|---|---|---|---|---|---|---|
| | $q_{5\%}$ | $q_{50\%}$ | $q_{95\%}$ | $q_{5\%}$ | $q_{50\%}$ | $q_{95\%}$ |
| Uniform | 0.184 | 0.331 | 0.494 | 0.581 | 0.773 | 0.905 |
| Radial stratification | 0.001 | 0.461 | 0.963 | 0.679 | 0.881 | 1.000 |
| Multi-corner stratification | 0.001 | 0.002 | 0.668 | 0.298 | 0.655 | 0.869 |

## S3 Details of MAP estimation and the Nyström approximation

This section collects the matrix identities and auxiliary expressions used in Section 4.4, including (i) gradients of the GP marginal log-likelihood, (ii) contributions of the *prioris* to the MAP objective, and (iii) efficient formulas (log-determinant and linear-system solves) under the Nyström approximation.

### S3.1 Matrix identities used

Let $\mathbf{A}(\theta)$ be a symmetric positive definite matrix depending on $\theta$. We will use the standard identities:

**Derivative of the log-determinant.**

$$\frac{\partial}{\partial \theta} \log \det(\mathbf{A}) = \operatorname{tr}\Big(\mathbf{A}^{-1} \frac{\partial \mathbf{A}}{\partial \theta}\Big). \tag{32}$$

**Derivative of the inverse.**

$$\frac{\partial \mathbf{A}^{-1}}{\partial \theta} = -\mathbf{A}^{-1} \Big(\frac{\partial \mathbf{A}}{\partial \theta}\Big) \mathbf{A}^{-1}. \tag{33}$$

**Trace form for a quadratic product.** For $\mathbf{y} \in \mathbb{R}^n$,

$$\mathbf{y}^\top \mathbf{A}^{-1} \Big(\frac{\partial \mathbf{A}}{\partial \theta}\Big) \mathbf{A}^{-1} \mathbf{y} = \operatorname{tr}\Big(\mathbf{A}^{-1} \mathbf{y}\mathbf{y}^\top \mathbf{A}^{-1} \frac{\partial \mathbf{A}}{\partial \theta}\Big).$$

### S3.2 Gradient of the GP marginal log-likelihood

In the regression model with independent Gaussian noise,

$$\mathbf{y} \mid \mathbf{X}, \theta \sim \mathcal{N}(\mathbf{0}, \widetilde{\mathbf{K}}_\theta), \qquad \widetilde{\mathbf{K}}_\theta = \mathbf{K}_\theta + \sigma_\epsilon^2 \mathbf{I}.$$

The marginal log-likelihood is

$$\log p(\mathbf{y} \mid \mathbf{X}, \theta) = -\frac{1}{2} \mathbf{y}^\top \widetilde{\mathbf{K}}_\theta^{-1} \mathbf{y} - \frac{1}{2} \log \det(\widetilde{\mathbf{K}}_\theta) - \frac{n}{2} \log(2\pi). \tag{34}$$

Define $\boldsymbol{\alpha} := \widetilde{\mathbf{K}}_\theta^{-1} \mathbf{y}$. Applying (32)–(33), we obtain the standard form:

$$\frac{\partial}{\partial \theta_j} \log p(\mathbf{y} \mid \mathbf{X}, \theta) = \frac{1}{2} \operatorname{tr}\Big[\big(\boldsymbol{\alpha}\boldsymbol{\alpha}^\top - \widetilde{\mathbf{K}}_\theta^{-1}\big) \frac{\partial \widetilde{\mathbf{K}}_\theta}{\partial \theta_j}\Big], \tag{35}$$

and therefore, for the *negative* log-likelihood,

$$\frac{\partial}{\partial \theta_j}\Big(-\log p(\mathbf{y} \mid \mathbf{X}, \theta)\Big) = \frac{1}{2}\,\mathrm{tr}\Big[(\widetilde{\mathbf{K}}_\theta^{-1} - \boldsymbol{\alpha}\boldsymbol{\alpha}^\top)\,\frac{\partial \widetilde{\mathbf{K}}_\theta}{\partial \theta_j}\Big]. \tag{36}$$

### S3.3 Derivatives of the approximate kernel matrix

In the reduced model used in the paper,

$$\mathbf{K}_\theta = \sigma_b^2\,\mathbf{1}\mathbf{1}^\top + \sigma_v^2\Big[w\,\mathbf{K}_{\mathrm{smooth}}(\sigma_a^2, \sigma_u^2) + (1-w)\,\mathbf{K}_{\mathrm{angular}}(\sigma_a^2, \sigma_u^2, \alpha)\Big], \qquad \widetilde{\mathbf{K}}_\theta = \mathbf{K}_\theta + \sigma_\epsilon^2\mathbf{I}. \tag{37}$$

The most frequently used matrix derivatives are:

**Noise.**

$$\frac{\partial \widetilde{\mathbf{K}}_\theta}{\partial \sigma_\epsilon^2} = \mathbf{I}. \tag{38}$$

**Constant term.**

$$\frac{\partial \widetilde{\mathbf{K}}_\theta}{\partial \sigma_b^2} = \mathbf{1}\mathbf{1}^\top. \tag{39}$$

**Overall kernel scale.**

$$\frac{\partial \widetilde{\mathbf{K}}_\theta}{\partial \sigma_v^2} = w\,\mathbf{K}_{\mathrm{smooth}} + (1-w)\,\mathbf{K}_{\mathrm{angular}}. \tag{40}$$

**Mixing weight.**

$$\frac{\partial \widetilde{\mathbf{K}}_\theta}{\partial w} = \sigma_v^2(\mathbf{K}_{\mathrm{smooth}} - \mathbf{K}_{\mathrm{angular}}). \tag{41}$$

**Parameter $\alpha$ (only in the angular component).**

$$\frac{\partial \widetilde{\mathbf{K}}_\theta}{\partial \alpha} = \sigma_v^2(1-w)\,\frac{\partial \mathbf{K}_{\mathrm{angular}}}{\partial \alpha}. \tag{42}$$

In the case where the inner LeakyReLU term is written as

$$K_{\mathrm{angular}}(\mathbf{x}, \mathbf{x}') = \sigma_z\sigma_{z'}\Big[\alpha\,\rho + (1-\alpha)^2\,S(\rho)\Big], \qquad S(\rho) = \frac{1}{2\pi}\Big(\sqrt{1-\rho^2} + \rho(\pi - \arccos\rho)\Big),$$

we have, pointwise,

$$\frac{\partial}{\partial \alpha}K_{\mathrm{angular}}(\mathbf{x}, \mathbf{x}') = \sigma_z\sigma_{z'}\Big[\rho - 2(1-\alpha)\,S(\rho)\Big],$$

and therefore $[\partial\mathbf{K}_{\mathrm{angular}}/\partial\alpha]_{ij}$ is obtained by evaluating the expression above at $(\mathbf{x}_i, \mathbf{x}_j)$.

**Internal parameters $(\sigma_a^2, \sigma_u^2)$.** The terms $\mathbf{K}_{\mathrm{smooth}}(\sigma_a^2, \sigma_u^2)$ and $\mathbf{K}_{\mathrm{angular}}(\sigma_a^2, \sigma_u^2, \alpha)$ depend on $(\sigma_a^2, \sigma_u^2)$ through $\sigma_z(\mathbf{x})$, $\sigma_{z'}(\mathbf{x}')$, and $\rho(\mathbf{x}, \mathbf{x}')$. Thus,

$$\frac{\partial \widetilde{\mathbf{K}}_\theta}{\partial \sigma_a^2} = \sigma_v^2\Big[w\,\frac{\partial \mathbf{K}_{\mathrm{smooth}}}{\partial \sigma_a^2} + (1-w)\,\frac{\partial \mathbf{K}_{\mathrm{angular}}}{\partial \sigma_a^2}\Big], \qquad \frac{\partial \widetilde{\mathbf{K}}_\theta}{\partial \sigma_u^2} = \sigma_v^2\Big[w\,\frac{\partial \mathbf{K}_{\mathrm{smooth}}}{\partial \sigma_u^2} + (1-w)\,\frac{\partial \mathbf{K}_{\mathrm{angular}}}{\partial \sigma_u^2}\Big]. \tag{43}$$

In the code, these derivatives are computed via automatic differentiation from the closed-form expressions for $K_{\mathrm{smooth}}$ and $K_{\mathrm{angular}}$ (making it unnecessary to spell out the full chain rule here, which is lengthy).

### S3.3.1 Gradients of the *prioris* in the MAP loss

The MAP loss in the main text is

$$\mathcal{L}_{\text{MAP}}(\theta) = \underbrace{-\log p(\mathbf{y} \mid \mathbf{X}, \theta)}_{\text{GP NLL}} + \underbrace{\big(-\log p(\theta)\big)}_{\text{penalty (prioris)}}.$$

**Inverse-Gamma *priori* for variances.** If $\sigma_q^2 \sim \text{Inv-Gamma}(a_q, b_q)$, then (ignoring constants)

$$-\log p(\sigma_q^2) = (a_q + 1)\log \sigma_q^2 + \frac{b_q}{\sigma_q^2},$$

and

$$\frac{\partial}{\partial \sigma_q^2}\big(-\log p(\sigma_q^2)\big) = \frac{a_q + 1}{\sigma_q^2} - \frac{b_q}{(\sigma_q^2)^2}. \tag{44}$$

**Beta *priori* for $\alpha$ and $w$.** If $\alpha \sim \text{Beta}(a_\alpha, b_\alpha)$, then (ignoring constants)

$$-\log p(\alpha) = -(a_\alpha - 1)\log \alpha - (b_\alpha - 1)\log(1 - \alpha),$$

and

$$\frac{\partial}{\partial \alpha}\big(-\log p(\alpha)\big) = -\frac{a_\alpha - 1}{\alpha} + \frac{b_\alpha - 1}{1 - \alpha}. \tag{45}$$

Analogously, for $w \sim \text{Beta}(a_w, b_w)$,

$$\frac{\partial}{\partial w}\big(-\log p(w)\big) = -\frac{a_w - 1}{w} + \frac{b_w - 1}{1 - w}. \tag{46}$$

## S3.4 Nyström approximation

MAP optimization for the GP requires repeated evaluations of $\widetilde{\mathbf{K}}_\theta^{-1}\mathbf{y}$ and $\log\det(\widetilde{\mathbf{K}}_\theta)$, where $\widetilde{\mathbf{K}}_\theta = \mathbf{K}_\theta + \sigma_\epsilon^2 \mathbf{I}_n$. Since an exact factorization of an $n \times n$ matrix costs $\mathcal{O}(n^3)$, we adopt the Nyström approximation (Banerjee et al., 2013) to make inference scalable.

We call *anchors* a subset of $r \ll n$ training points used to represent the kernel geometry in a low-dimensional subspace. Let $S \subset \{1, \ldots, n\}$ be the set of anchor indices with $|S| = r$. Define the Nyström blocks (built from $\mathbf{K}_\theta$):

$$\mathbf{C} := \mathbf{K}_{\theta,:S} \in \mathbb{R}^{n \times r}, \qquad \mathbf{W} := \mathbf{K}_{\theta,SS} \in \mathbb{R}^{r \times r}.$$

Then the Nyström approximation is

$$\mathbf{K}_\theta \;\approx\; \mathbf{C}\,\mathbf{W}^{-1}\mathbf{C}^\top, \qquad \text{hence} \qquad \widetilde{\mathbf{K}}_\theta = \mathbf{K}_\theta + \sigma_\epsilon^2 \mathbf{I}_n \;\approx\; \sigma_\epsilon^2 \mathbf{I}_n + \mathbf{C}\,\mathbf{W}^{-1}\mathbf{C}^\top. \tag{47}$$

With this construction, the dominant costs typically reduce to $\mathcal{O}(nr^2)$ (instead of $\mathcal{O}(n^3)$), enabling efficient approximations of $\log\det(\widetilde{\mathbf{K}}_\theta)$ and solutions of linear systems $\widetilde{\mathbf{K}}_\theta \mathbf{u} = \mathbf{y}$ within the MAP loop.

**Anchor selection.** The anchor set $S$ can be chosen in several ways, including random sampling, *k-means++* initialization (or centroids obtained via $k$-means) (Arthur and Vassilvitskii, 2007), or randomized projections that approximate the column space of $\mathbf{K}_\theta$ (Rahimi and Recht, 2007; Halko et al., 2011). In this work we use two practical rules, depending on the experimental design: (i) FIRST, where $S = \{1, \ldots, r\}$ (useful in simulation pipelines where the data-generation order is controlled); and (ii) KMEANS++, where we initialize $r$ centroids with K-MEANS++ (optionally refine with a few K-MEANS iterations) and set $S$ as the indices of the training points closest to the resulting centroids. Rule (ii) follows common practice in the literature, often producing anchors that better represent the geometry of the dataset.

**Computational details.** The reduced-dimension formulas for (i) solving $\widetilde{\mathbf{K}}_\theta \boldsymbol{\alpha} = \mathbf{y}$ and (ii) computing $\log\det(\widetilde{\mathbf{K}}_\theta)$ using only $r \times r$ factorizations/solves are given in Appendix S4. Algorithm S1 describes anchor selection, and Algorithm S2 summarizes the Nyström routine used inside MAP.

# S4 Nyström auxiliary routines (pseudocode)

**Algorithm S1** Anchor selection for Nyström (*first* or *k-means++*)

**Require:** Input set $\mathbf{X} = \{\mathbf{x}_i\}_{i=1}^n$, rank $r \ll n$, method ANCHOR $\in \{$FIRST, KMEANS++$\}$.
**Ensure:** Anchor indices $S \subset \{1, \ldots, n\}$ with $|S| = r$.

**if** ANCHOR = FIRST **then**
    $S \leftarrow \{1, 2, \ldots, r\}$.
**else** ▷ ANCHOR = KMEANS++
    Run *k-means++* to initialize $r$ centroids over $\{\mathbf{x}_i\}_{i=1}^n$.
    (Optional) Refine the centroids with a few iterations of standard $k$-means.
    For each centroid, select the index of the closest point in $\mathbf{X}$.
    Let $S$ be the set of these $r$ indices (if duplicates occur, fill with the next closest points).
**end if**
**return** $S$.

**Algorithm S2** Nyström for $\widetilde{\mathbf{K}}_\theta^{-1}\mathbf{y}$ and $\log\det(\widetilde{\mathbf{K}}_\theta)$ in MAP optimization

**Require:** Data $(\mathbf{X}, \mathbf{y})$ with $n$ points; parameters $\theta$ (define $K_\theta$); noise $\sigma_\epsilon^2$; anchors $S$ with $|S| = r$; *jitter* $\lambda > 0$ (small).
**Ensure:** Approximations $\boldsymbol{\alpha} \approx \widetilde{\mathbf{K}}_\theta^{-1}\mathbf{y}$ and $\log\det(\widetilde{\mathbf{K}}_\theta)$.

**(1) Kernel submatrices)**
Compute $\mathbf{C} \leftarrow \mathbf{K}_{\theta,:S} \in \mathbb{R}^{n\times r}$ and $\mathbf{W} \leftarrow \mathbf{K}_{\theta,SS} \in \mathbb{R}^{r\times r}$.
**(2) Stabilization and factorization)**
$\mathbf{W} \leftarrow \mathbf{W} + \lambda \mathbf{I}_r$ ▷ ensures numerical SPD
Compute the Cholesky factorization: $\mathbf{W} = \mathbf{L}\mathbf{L}^\top$.
**(3) Low-rank factor)**
$\boldsymbol{\Phi} \leftarrow \mathbf{C}\,\mathbf{L}^{-\top} \in \mathbb{R}^{n\times r}$.
**(4) Reduced system)**
$\mathbf{A} \leftarrow \sigma_\epsilon^2 \mathbf{I}_r + \boldsymbol{\Phi}^\top\boldsymbol{\Phi} \in \mathbb{R}^{r\times r}$
$\mathbf{b} \leftarrow \boldsymbol{\Phi}^\top\mathbf{y} \in \mathbb{R}^r$
Solve $\mathbf{A}\mathbf{v} = \mathbf{b}$ via Cholesky in $r \times r$.
**(5) Recover $\boldsymbol{\alpha}$)**
$\boldsymbol{\alpha} \leftarrow \frac{1}{\sigma_\epsilon^2}\left(\mathbf{y} - \boldsymbol{\Phi}\mathbf{v}\right)$.
**(6) Approximate log-determinant)**
Compute $\log\det(\mathbf{A})$ via Cholesky $\mathbf{A} = \mathbf{R}\mathbf{R}^\top$: $\log\det(\mathbf{A}) = 2\sum_{i=1}^r \log R_{ii}$.
Set

$$\log\det(\widetilde{\mathbf{K}}_\theta) \;\approx\; (n-r)\log\sigma_\epsilon^2 + \log\det(\mathbf{A}).$$

**return** $(\boldsymbol{\alpha},\ \log\det(\widetilde{\mathbf{K}}_\theta))$.

# S5 Details of the sequential *Vecchia*-type simulation

This section describes the procedure used to generate $f(\tilde{\mathbf{x}}_i)$ in regimes with large $n$, avoiding the cubic cost associated with exact sampling from $\mathbf{f} \sim \mathcal{N}(0, \mathbf{K})$. The method approximates the joint distribution by a sequence of local conditionals, following the *Vecchia* idea.

## S5.1 Exact initial block

Let $\tilde{\mathbf{x}}_1, \ldots, \tilde{\mathbf{x}}_n$ be the inputs in the scenario. We choose $N_{\text{init}} \ll n$ and sample the first values exactly:

$$\mathbf{f}_{1:N_{\text{init}}} \sim \mathcal{N}(\mathbf{0},\, \mathbf{K}_{\text{init}})\,, \qquad \mathbf{K}_{\text{init}} = \left[K_{\text{mix}}(\tilde{\mathbf{x}}_i, \tilde{\mathbf{x}}_j)\right]_{1\le i,j\le N_{\text{init}}}.$$

Sampling is performed via a Cholesky factorization:

$$\mathbf{K}_{\text{init}} = \mathbf{L}\mathbf{L}^\top, \qquad \mathbf{f}_{1:N_{\text{init}}} = \mathbf{L}\boldsymbol{\xi}, \qquad \boldsymbol{\xi} \sim \mathcal{N}(\mathbf{0}, \mathbf{I}).$$

## S5.2 Sequential step via local conditionals

For each $j = N_{\text{init}} + 1, \ldots, n$, we select the $N_{\text{viz}}$ nearest neighbors of $\tilde{\mathbf{x}}_j$ among the previous indices $\{1, \ldots, j-1\}$, using Euclidean distance. Denote by $\mathcal{N}_j = \{i_1, \ldots, i_{N_{\text{viz}}}\}$ the set of neighbor indices and define:

$$\mathbf{K}_{\mathcal{N}_j,\mathcal{N}_j} = \left[K_{\text{mix}}(\tilde{\mathbf{x}}_{i_a}, \tilde{\mathbf{x}}_{i_b})\right]_{a,b=1}^{N_{\text{viz}}}, \qquad \mathbf{k}_{j,\mathcal{N}_j} = \left(K_{\text{mix}}(\tilde{\mathbf{x}}_j, \tilde{\mathbf{x}}_{i_1}), \ldots, K_{\text{mix}}(\tilde{\mathbf{x}}_j, \tilde{\mathbf{x}}_{i_{N_{\text{viz}}}})\right),$$

and $\mathbf{f}_{\mathcal{N}_j} = (f_{i_1}, \ldots, f_{i_{N_{\text{viz}}}})^\top$. The conditional distribution of $f_j = f(\tilde{\mathbf{x}}_j)$ given $\mathbf{f}_{\mathcal{N}_j}$ is univariate Gaussian:

$$f_j \mid \mathbf{f}_{\mathcal{N}_j} \sim \mathcal{N}(\mu_j, \sigma_j^2),$$

with

$$\mu_j = \mathbf{k}_{j,\mathcal{N}_j} \mathbf{K}_{\mathcal{N}_j,\mathcal{N}_j}^{-1} \mathbf{f}_{\mathcal{N}_j}, \qquad \sigma_j^2 = K_{\text{mix}}(\tilde{\mathbf{x}}_j, \tilde{\mathbf{x}}_j) - \mathbf{k}_{j,\mathcal{N}_j} \mathbf{K}_{\mathcal{N}_j,\mathcal{N}_j}^{-1} \mathbf{k}_{j,\mathcal{N}_j}^\top. \tag{48}$$

A sample is then generated as

$$f_j = \mu_j + \sqrt{\sigma_j^2}\, \xi_j, \qquad \xi_j \sim \mathcal{N}(0, 1).$$

## S5.3 Technical note: use of Cholesky factorization

At all stages, we avoid computing inverses explicitly. To compute terms such as $\mathbf{K}^{-1}\mathbf{v}$ in (48), we use $\mathbf{K} = \mathbf{L}\mathbf{L}^\top$ and solve triangular systems:

$$\mathbf{K}^{-1}\mathbf{v} = (\mathbf{L}^\top)^{-1}(\mathbf{L}^{-1}\mathbf{v}),$$

which improves numerical stability and reduces cost. This practice is consistent with standard recommendations in GPs Rasmussen and Williams (2006).

In this sense, by combining the exact initial block and the local conditionals, we obtain an approximate construction of $\mathbf{f} \approx \mathcal{N}(\mathbf{0}, \mathbf{K})$ that preserves local dependencies typical of GPs, with complexity controlled by $N_{\text{init}}$ and $N_{\text{viz}}$. Finally, we generate the observations as

$$y(\tilde{\mathbf{x}}_j) = f(\tilde{\mathbf{x}}_j) + \varepsilon(\tilde{\mathbf{x}}_j), \qquad \varepsilon(\tilde{\mathbf{x}}_j) \overset{iid}{\sim} \mathcal{N}(0, \sigma_\varepsilon^2),$$

with $\sigma_\varepsilon^2$ defined by the reproducible rule:

$$\sigma_\varepsilon^2 = \eta\, \overline{K}, \qquad \overline{K} = \frac{1}{n}\sum_{i=1}^{n} K_{\text{mix}}(\tilde{\mathbf{x}}_i, \tilde{\mathbf{x}}_i), \tag{49}$$

**Note.** In all sequential-simulation experiments, we set $N_{\text{viz}} = 500$.

## S5.4 Model evaluation metrics

After training the model on $\mathcal{D}_{\text{train}} = \{(\mathbf{x}_i, y_i)\}_{i=1}^{N}$, we compute predictions on the test set $\mathcal{D}_{\text{test}} = \{(\mathbf{x}_i, y_i)\}_{i=N+1}^{n}$, with $N_{\text{test}} = n - N$. Given MAP estimates of the hyperparameters, the GP predictive distribution for each test input is

$$Y_i \mid \mathcal{D}_{\text{train}}, \mathbf{x}_i \sim \mathcal{N}(\hat{y}_i, \hat{\sigma}_i^2), \qquad i = N+1, \ldots, n,$$

where $\hat{y}_i = \mathbb{E}[Y_i \mid \mathcal{D}_{\text{train}}, \mathbf{x}_i]$ and $\hat{\sigma}_i^2 = \text{Var}(Y_i \mid \mathcal{D}_{\text{train}}, \mathbf{x}_i)$. We use the following metrics.

**Mean absolute error (MAE).**

$$\text{MAE} = \frac{1}{N_{\text{test}}} \sum_{i=N+1}^{n} |y_i - \hat{y}_i|\,.$$

Its relative version (when $y_i \neq 0$) is

$$\text{MAE}_R = \frac{1}{N_{\text{test}}} \sum_{i=N+1}^{n} \left| \frac{y_i - \hat{y}_i}{y_i} \right|.$$

**Mean squared error (MSE) and root mean squared error (RMSE).**

$$\mathrm{MSE} = \frac{1}{N_{\text{test}}} \sum_{i=N+1}^{n} (y_i - \hat{y}_i)^2, \qquad \mathrm{RMSE} = \sqrt{\mathrm{MSE}}.$$

Relative versions (when $y_i \neq 0$) are

$$\mathrm{MSE}_R = \frac{1}{N_{\text{test}}} \sum_{i=N+1}^{n} \left(\frac{y_i - \hat{y}_i}{y_i}\right)^2, \qquad \mathrm{RMSE}_R = \sqrt{\mathrm{MSE}_R}.$$

**Expected squared error (ESE).** For each test point, we define the expected squared error under the predictive distribution:

$$\mathrm{ESE}_i = \mathbb{E}\Big[(Y_i - y_i)^2 \mid \mathcal{D}_{\text{train}}, \mathbf{x}_i\Big] = \hat{\sigma}_i^2 + (\hat{y}_i - y_i)^2.$$

The relative version (when $y_i \neq 0$) is

$$\mathrm{ESE}_{i,R} = \mathbb{E}\left[\left(\frac{Y_i - y_i}{y_i}\right)^2 \,\middle|\, \mathcal{D}_{\text{train}}, \mathbf{x}_i\right] = \frac{1}{y_i^2}\Big(\hat{\sigma}_i^2 + (\hat{y}_i - y_i)^2\Big).$$

**Mean expected squared error (MESE).**

$$\mathrm{MESE} = \frac{1}{N_{\text{test}}} \sum_{i=N+1}^{n} \mathrm{ESE}_i, \qquad \mathrm{MESE}_R = \frac{1}{N_{\text{test}}} \sum_{i=N+1}^{n} \mathrm{ESE}_{i,R}.$$

**Standard deviation of the expected squared error (SDESE).**

$$\mathrm{SDESE} = \left(\frac{1}{N_{\text{test}} - 1} \sum_{i=N+1}^{n} (\mathrm{ESE}_i - \mathrm{MESE})^2\right)^{1/2},$$

$$\mathrm{SDESE}_R = \left(\frac{1}{N_{\text{test}} - 1} \sum_{i=N+1}^{n} (\mathrm{ESE}_{i,R} - \mathrm{MESE}_R)^2\right)^{1/2}.$$

**Normalized metrics for real datasets.** For real datasets, the model is trained on the standardized target $\tilde{y} = (y - \mu_y)/\sigma_y$ computed on the training set. We report errors both on the original scale (after de-standardizing predictions) and on the standardized scale, e.g., $\mathrm{MAE}_z = \mathrm{MAE}/\sigma_y$ and $\mathrm{RMSE}_z = \mathrm{RMSE}/\sigma_y$.

# S6 Supplementary Experiments

This appendix reports the additional experimental details and full tables omitted from the main paper for space. It includes: (i) the complete list of simulation scenarios (C1–C8) and replication summaries; (ii) full results for both training protocols (fixed-cost and EarlyStopping) with both Nyström anchor strategies; and (iii) extended real-data tables, including normalized metrics and the full Nyström-rank grid on the full *YearPredictionMSD* benchmark.

## S6.1 Full simulation design (C1–C8)

Table 3 lists the eight simulated scenarios obtained by combining sample size $n \in \{10k, 20k, 50k\}$, dimension $I \in \{20, 80\}$, and (for $n = 50k$) uniform vs. stratified input designs. In all cases, outputs follow

$$y(\tilde{x}) = f(\tilde{x}) + \varepsilon, \qquad f \sim \mathcal{GP}(0, K_{\text{mix}}), \quad \varepsilon \overset{iid}{\sim} \mathcal{N}(0, \sigma_\varepsilon^2),$$

with nugget calibrated as $\sigma_\varepsilon^2 = \eta \overline{K}$, $\eta = 0.04$, and $\overline{K} = \frac{1}{n}\sum_{i=1}^{n} K_{\text{mix}}(\tilde{x}_i, \tilde{x}_i)$.

## S6.2 Replication study (C1)

To quantify variability due to the latent-process and noise realization, we run $R = 20$ replications of scenario C1, keeping $\tilde{\mathbf{X}}$ fixed and varying only the output seed. Table S2 reports descriptive statistics of $y$ and simulation time per replication.

Table S2: Replications of scenario C1. The nugget is constant within the scenario, with $\overline{K} = 2.132745$ and $\sigma_\varepsilon = 0.292078$. We report descriptive statistics of $y$ and the simulation time per replication.

| **Rep.** | **Time (s)** | $\bar{y}$ | **sd**$(y)$ | $q_{0.25}$ | $q_{0.50}$ | $q_{0.75}$ |
|---|---|---|---|---|---|---|
| 1 | 37.743791 | -2.762978 | 0.758659 | -3.285670 | -2.761005 | -2.247959 |
| 2 | 33.173773 | -1.483116 | 0.747860 | -1.998242 | -1.500517 | -0.965862 |
| 3 | 31.540114 | 0.297776 | 0.800180 | -0.240019 | 0.299212 | 0.850236 |
| 4 | 32.523281 | -0.920560 | 0.936782 | -1.574556 | -0.925901 | -0.271994 |
| 5 | 32.068839 | 1.339821 | 1.018936 | 0.635007 | 1.332660 | 2.036681 |
| 6 | 38.222421 | -1.869241 | 0.871449 | -2.464713 | -1.868421 | -1.269481 |
| 7 | 39.741229 | -0.767632 | 0.738668 | -1.262645 | -0.767888 | -0.275450 |
| 8 | 38.047494 | 0.632211 | 0.958910 | -0.028639 | 0.619439 | 1.292294 |
| 9 | 32.062171 | -0.835366 | 1.010224 | -1.536437 | -0.848563 | -0.131389 |
| 10 | 32.255612 | -1.979346 | 0.876620 | -2.571465 | -1.974819 | -1.370490 |
| 11 | 32.263780 | -0.171990 | 0.821994 | -0.738855 | -0.172324 | 0.389725 |
| 12 | 31.336121 | -0.954957 | 0.723242 | -1.442938 | -0.957556 | -0.459980 |
| 13 | 32.144726 | 0.918489 | 0.799278 | 0.380536 | 0.927228 | 1.469647 |
| 14 | 31.571111 | 0.327178 | 0.909407 | -0.302598 | 0.335681 | 0.958325 |
| 15 | 32.024871 | -1.235445 | 0.883276 | -1.835635 | -1.244995 | -0.623431 |
| 16 | 31.591529 | 0.402182 | 1.033072 | -0.314244 | 0.380714 | 1.088846 |
| 17 | 32.016006 | 0.347500 | 0.737527 | -0.154734 | 0.356702 | 0.859837 |
| 18 | 32.346621 | 1.339351 | 0.882890 | 0.726023 | 1.340382 | 1.956343 |
| 19 | 31.997308 | 1.650710 | 0.866563 | 1.064933 | 1.657125 | 2.251200 |
| 20 | 31.706423 | 1.331327 | 0.800550 | 0.781486 | 1.333523 | 1.879761 |

For completeness, Table 6 summarizes test metrics and MAP estimates across replications for Protocol 1 with Nyström ($r = 500$) and $k$-means anchors.

## S6.3 Full Protocol 2 results (EarlyStopping)

## S6.4 Degenerate mixture cases

Table S5 reports $\Delta$RMSE relative to $K_{\text{mix}}$ fit with EarlyStopping:

$$\Delta\text{RMSE} = \text{RMSE}(w \text{ fixed}) - \text{RMSE}(K_{\text{mix}}{+}ES),$$

so $\Delta > 0$ indicates worse performance than the learned mixture.

Table S3: Protocol 1: MAP estimates under two anchor-selection strategies. The nugget is reported as variance $\hat{\sigma}_\epsilon^2$.

| Scenario | Anchors | $\hat{\sigma}_b^2$ | $\hat{\sigma}_v^2$ | $\hat{\sigma}_u^2$ | $\hat{\sigma}_a^2$ | $\hat{\alpha}$ | $\hat{w}$ | $\hat{\sigma}_\epsilon^2$ |
|---|---|---|---|---|---|---|---|---|
| C1 | first | 1.025371 | 0.980080 | 0.981301 | 0.994972 | 0.508588 | 0.495693 | $8.56 \times 10^{-2}$ |
| C1 | $k$-means | 1.026216 | 0.987962 | 0.995776 | 0.987359 | 0.508575 | 0.496666 | $8.29 \times 10^{-2}$ |
| C2 | first | 1.015887 | 1.031211 | 1.030972 | 0.968986 | 0.487482 | 0.512434 | $1.64 \times 10^{-1}$ |
| C2 | $k$-means | 1.028323 | 1.032194 | 1.032033 | 0.968549 | 0.487544 | 0.511323 | $1.63 \times 10^{-1}$ |
| C3 | first | 1.028055 | 0.971542 | 0.972107 | 0.983965 | 0.511472 | 0.491441 | $8.64 \times 10^{-2}$ |
| C3 | $k$-means | 1.023113 | 0.974400 | 0.976894 | 0.996529 | 0.510373 | 0.490998 | $8.18 \times 10^{-2}$ |
| C4 | first | 0.999669 | 1.031572 | 1.031348 | 0.968746 | 0.487415 | 0.511870 | $1.64 \times 10^{-1}$ |
| C4 | $k$-means | 1.018052 | 1.031881 | 1.031831 | 0.968938 | 0.487784 | 0.509282 | $1.63 \times 10^{-1}$ |
| C5 | first | 1.028704 | 0.971421 | 0.971586 | 0.994188 | 0.511165 | 0.490527 | $8.34 \times 10^{-2}$ |
| C5 | $k$-means | 1.025100 | 0.969336 | 0.969129 | 1.001332 | 0.511568 | 0.489583 | $8.21 \times 10^{-2}$ |
| C6 | first | 1.001530 | 1.031871 | 1.031808 | 0.969091 | 0.487441 | 0.512053 | $1.64 \times 10^{-1}$ |
| C6 | $k$-means | 1.014398 | 1.031409 | 1.031123 | 0.969269 | 0.487602 | 0.511393 | $1.64 \times 10^{-1}$ |
| C7 | first | 1.025906 | 0.971412 | 0.971880 | 1.002389 | 0.511691 | 0.489485 | $8.32 \times 10^{-2}$ |
| C7 | $k$-means | 1.024638 | 0.971043 | 0.972473 | 1.013075 | 0.512253 | 0.489012 | $8.33 \times 10^{-2}$ |
| C8 | first | 0.983979 | 1.031795 | 1.031675 | 0.968993 | 0.487443 | 0.512017 | $1.64 \times 10^{-1}$ |
| C8 | $k$-means | 1.018084 | 1.031796 | 1.031743 | 0.969018 | 0.487622 | 0.511714 | $1.64 \times 10^{-1}$ |

Table S4: Total time and test-set metrics under two anchor-selection strategies. Total time includes training and prediction.

| Scenario | Anchors | Total time (s) | MAE | MSE | RMSE | MESE | SDESE |
|---|---|---|---|---|---|---|---|
| C1 | first | 1.334 | 0.265983 | 0.112261 | 0.335053 | 0.236112 | 0.165608 |
| C1 | $k$-means | 2.155 | 0.263822 | 0.110102 | 0.331816 | 0.233065 | 0.161552 |
| C2 | first | 1.284 | 0.573294 | 0.504148 | 0.710034 | 0.892681 | 0.665183 |
| C2 | $k$-means | 2.514 | 0.534228 | 0.440660 | 0.663822 | 0.829185 | 0.585415 |
| C3 | first | 1.881 | 0.265764 | 0.110175 | 0.331926 | 0.233302 | 0.152864 |
| C3 | $k$-means | 2.137 | 0.264066 | 0.109563 | 0.331004 | 0.229287 | 0.153301 |
| C4 | first | 2.101 | 0.571924 | 0.515084 | 0.717694 | 0.903406 | 0.718319 |
| C4 | $k$-means | 2.334 | 0.562438 | 0.498106 | 0.705766 | 0.886464 | 0.707048 |
| C5 | first | 1.623 | 0.269528 | 0.114101 | 0.337789 | 0.233814 | 0.160743 |
| C5 | $k$-means | 2.408 | 0.267161 | 0.111680 | 0.334185 | 0.231012 | 0.159149 |
| C6 | first | 1.550 | 0.593175 | 0.562680 | 0.750120 | 0.950702 | 0.807495 |
| C6 | $k$-means | 3.511 | 0.566497 | 0.503485 | 0.709567 | 0.892490 | 0.718490 |
| C7 | first | 1.389 | 0.270088 | 0.115020 | 0.339146 | 0.234563 | 0.165507 |
| C7 | $k$-means | 2.592 | 0.270696 | 0.116113 | 0.340753 | 0.237124 | 0.168015 |
| C8 | first | 1.335 | 0.583224 | 0.537355 | 0.733045 | 0.927608 | 0.777588 |
| C8 | $k$-means | 1.395 | 0.581387 | 0.538477 | 0.733810 | 0.929836 | 0.774792 |

## S6.5 Additional results with *Early Stopping*

In this section, we report additional results using ES based on the NLL on the validation set. Training is stopped when the NLL fails to improve by more than $\delta$ for $P$ consecutive epochs, up to a maximum of $E_{\max}$ epochs. These results complement the main text and, overall, preserve the qualitative conclusions: (i) stability of the MAP fit, (ii) differences between anchor-selection strategies are more relevant in harder regimes, and (iii) a cost–accuracy trade-off driven by higher computational effort in more challenging settings.

Table S6 reports the MAP estimates with ES for *first* and *k-means*. The estimates remain stable, and $\hat{w}$ stays away from degenerate cases in most scenarios. Table S7 reports test-set metrics and total

Table S5: Degenerate cases: test-set RMSE difference relative to $K_{\text{mix}}$ fit with ES. We define $\Delta\text{RMSE} = \text{RMSE}(w \text{ fixed}) - \text{RMSE}(K_{\text{mix}}{+}ES)$, so $\Delta > 0$ indicates worse performance than $K_{\text{mix}}{+}ES$.

| Scenario | ΔRMSE ($w$=0 vs. mix+ES) | ΔRMSE ($w$=1 vs. mix+ES) |
|---|---|---|
| C1 | -0.0001 | +0.0073 |
| C2 | +0.0022 | +0.0057 |
| C3 | +0.0030 | +0.0101 |
| C4 | +0.0028 | +0.0056 |
| C5 | -0.0094 | +0.0000 |
| C6 | +0.0090 | -0.0009 |
| C7 | +0.0128 | +0.0173 |
| C8 | +0.0140 | -0.0095 |

Table S6: Protocol 2: MAP parameter estimates with ES under two anchor-selection strategies.

| Scenario | Anchors | $\hat{\sigma}_b^2$ | $\hat{\sigma}_v^2$ | $\hat{\sigma}_u^2$ | $\hat{\sigma}_a^2$ | $\hat{\alpha}$ | $\hat{w}$ | $\hat{\sigma}_\varepsilon^2$ |
|---|---|---|---|---|---|---|---|---|
| C1 | first | 1.000632 | 0.999368 | 0.999368 | 1.000632 | 0.499750 | 0.499750 | $8.51 \times 10^{-2}$ |
| C1 | $k$-means | 1.000632 | 1.000632 | 1.000632 | 0.999368 | 0.499750 | 0.500250 | $8.51 \times 10^{-2}$ |
| C2 | first | 1.063595 | 1.061767 | 1.061027 | 0.940711 | 0.476131 | 0.518270 | $1.77 \times 10^{-1}$ |
| C2 | $k$-means | 1.054798 | 1.065431 | 1.065326 | 0.938819 | 0.475053 | 0.513215 | $1.67 \times 10^{-1}$ |
| C3 | first | 1.000632 | 0.999368 | 0.999368 | 0.999368 | 0.500250 | 0.499750 | $8.51 \times 10^{-2}$ |
| C3 | $k$-means | 1.000632 | 0.999368 | 0.999368 | 1.000632 | 0.500250 | 0.499750 | $8.51 \times 10^{-2}$ |
| C4 | first | 1.065021 | 1.058914 | 1.057490 | 0.942075 | 0.480532 | 0.518081 | $1.78 \times 10^{-1}$ |
| C4 | $k$-means | 1.072058 | 1.082083 | 1.080863 | 0.922774 | 0.467914 | 0.517566 | $1.77 \times 10^{-1}$ |
| C5 | first | 1.000632 | 0.999368 | 0.999368 | 1.000632 | 0.500250 | 0.499750 | $8.51 \times 10^{-2}$ |
| C5 | $k$-means | 1.000632 | 0.999368 | 0.999368 | 1.000632 | 0.500250 | 0.499750 | $8.51 \times 10^{-2}$ |
| C6 | first | 1.039284 | 1.072502 | 1.071101 | 0.928890 | 0.471938 | 0.525394 | $1.82 \times 10^{-1}$ |
| C6 | $k$-means | 1.034433 | 1.064416 | 1.062903 | 0.936365 | 0.474339 | 0.520788 | $1.78 \times 10^{-1}$ |
| C7 | first | 1.000632 | 0.999368 | 0.999368 | 1.000632 | 0.500250 | 0.499750 | $8.51 \times 10^{-2}$ |
| C7 | $k$-means | 1.000632 | 0.999368 | 0.999368 | 1.000632 | 0.500250 | 0.499750 | $8.51 \times 10^{-2}$ |
| C8 | first | 1.068264 | 1.070736 | 1.069834 | 0.931383 | 0.472606 | 0.523457 | $1.82 \times 10^{-1}$ |
| C8 | $k$-means | 1.103498 | 1.093192 | 1.091510 | 0.911072 | 0.462990 | 0.533629 | $1.91 \times 10^{-1}$ |

time. As expected, in simpler scenarios training stops early, whereas in more challenging scenarios the total time increases substantially. In predictive terms, the procedure tends to concentrate computational effort where larger gains in generalization are more likely.

Overall, the ES results support the same qualitative picture reported in the main text. The MAP fit remains stable across scenarios and anchor choices (Table S6), with $\hat{w}$ consistently away from degenerate values, while the adaptive stopping rule primarily affects the effective computational budget. In particular, ES tends to allocate more training effort to harder regimes, where improvements in generalization are more likely, at the expense of increased total time (Table S7). These additional experiments therefore corroborate that our conclusions are not an artifact of the fixed-epoch protocol, but persist under an alternative and widely used training criterion.

Table S7: Total time and test-set metrics under two anchor-selection strategies.

| Scenario | Anchors | Total time (s) | MAE | MSE | RMSE | MESE | SDESE |
|---|---|---|---|---|---|---|---|
| C1 | first | 0.580 | 0.263083 | 0.107923 | 0.328516 | 0.233985 | 0.152893 |
| C1 | $k$-means | 0.577 | 0.263046 | 0.109756 | 0.331294 | 0.236683 | 0.162246 |
| C2 | first | 7.268 | 0.535882 | 0.448688 | 0.669842 | 0.879033 | 0.615846 |
| C2 | $k$-means | 8.023 | 0.539868 | 0.448492 | 0.669695 | 0.870721 | 0.579662 |
| C3 | first | 0.791 | 0.266499 | 0.110782 | 0.332839 | 0.236913 | 0.155212 |
| C3 | $k$-means | 0.624 | 0.267808 | 0.113895 | 0.337483 | 0.240882 | 0.161825 |
| C4 | first | 7.228 | 0.552473 | 0.477697 | 0.691157 | 0.903436 | 0.673074 |
| C4 | $k$-means | 8.080 | 0.569828 | 0.501686 | 0.708298 | 0.949708 | 0.678545 |
| C5 | first | 1.013 | 0.266409 | 0.112144 | 0.334879 | 0.237937 | 0.161910 |
| C5 | $k$-means | 1.013 | 0.274136 | 0.117728 | 0.343116 | 0.245070 | 0.166490 |
| C6 | first | 9.857 | 0.572213 | 0.515220 | 0.717788 | 0.959397 | 0.727788 |
| C6 | $k$-means | 12.303 | 0.568623 | 0.506527 | 0.711707 | 0.940060 | 0.723270 |
| C7 | first | 1.109 | 0.272383 | 0.116194 | 0.340873 | 0.241956 | 0.163225 |
| C7 | $k$-means | 1.088 | 0.268451 | 0.114075 | 0.337750 | 0.241397 | 0.166022 |
| C8 | first | 13.507 | 0.570334 | 0.514463 | 0.717261 | 0.958192 | 0.755247 |
| C8 | $k$-means | 21.778 | 0.595730 | 0.566103 | 0.752398 | 1.042524 | 0.817726 |

# References


David Arthur and Sergei Vassilvitskii. **k-means++: The Advantages of Careful Seeding**. In *Proceedings of the Eighteenth Annual ACM-SIAM Symposium on Discrete Algorithms (SODA)*, pages 1027–1035, Philadelphia, PA, USA, 2007. SIAM. doi: 10.1145/1283383.1283494.

Anindya Banerjee, David B. Dunson, and Surya T. Tokdar. **Efficient Gaussian process regression for large datasets**. *Biometrika*, 100(1):75–89, 2013. doi: 10.1093/biomet/ass068.

Nathan Halko, Per-Gunnar Martinsson, and Joel A. Tropp. **Finding Structure with Randomness: Probabilistic Algorithms for Constructing Approximate Matrix Decompositions**. *SIAM Review*, 53(2):217–288, 2011.

Jaehoon Lee, Yasaman Bahri, Roman Novak, Samuel S. Schoenholz, Jeffrey Pennington, and Jascha Sohl-Dickstein. **Deep Neural Networks as Gaussian Processes**. In *International Conference on Learning Representations (ICLR)*. OpenReview.net, 2018. URL `https://openreview.net/forum?id=B1EA-M-0Z`.

Radford M. Neal. ***Bayesian Learning for Neural Networks***, volume 118 of *Lecture Notes in Statistics*. Springer, New York, 1996.

Roman Novak, Lechao Xiao, Jiri Hron, Jaehoon Lee, Alexander A. Alemi, Jascha Sohl-Dickstein, and Samuel S. Schoenholz. **Neural Tangents: Fast and Easy Infinite Neural Networks in Python**. *International Conference on Learning Representations*, 2020. URL `https://github.com/google/neural-tangents`.

Ali Rahimi and Benjamin Recht. **Random Features for Large-Scale Kernel Machines**. In John C. Platt, Daphne Koller, Yoram Singer, and Sam Roweis, editors, *Advances in Neural Information Processing Systems (NeurIPS)*, volume 20, pages 1177–1184. Curran Associates, Inc., 2007. URL `https://papers.nips.cc/paper_files/paper/2007/hash/013a006f03dbc5392effeb8f18fda755-Abstract.html`.

Carl Edward Rasmussen and Christopher K. I. Williams. ***Gaussian Processes for Machine Learning***. MIT Press, Cambridge, MA, USA, 2006. ISBN 026218253X.

Christopher K. I. Williams. **Computing with Infinite Networks**. *Neural Computation*, 10(5): 1203–1216, 1997.
